# Supplementary material for: Swarmodroid & AMPy: Reconfigurable Bristle-Bots and Software Package for Robotic Active Matter Studies
Source: arXiv:2305.13510 source file (2025-11-05)
Supplement: Supplementary file 1 [file SupplementaryPreCompiled.pdf]

# Supplementary Information:
# Swarmodroid 1.0: A Modular Bristle-Bot Platform for Robotic Active Matter Studies

## CONTENTS


S1. Power consumption of robots and battery characterization 2

S2. Algorithm of the robot firmware 4
- S2.1. The `main` procedure 4
- S2.2. 8-bit Timer/Counter 7
- S2.3. Pin change interrupt ISR 8

S3. Firmware reference 11
- S3.1. Global variables 11
- S3.2. Macro definitions: hardware-related constants 13
- S3.3. Macro definitions: inline functions 14
- S3.4. Macro definitions: definitions introduced for code clarity 17
- S3.5. Remote control constants 19
- S3.6. `measure_and_show_battery_idle_voltage` function 20
- S3.7. `main` function 20
- S3.8. Timer/Counter overflow interrupt service routine 24
- S3.9. ADC conversion complete interrupt service routine 24
- S3.10. Pin change interrupt service routine 25

References 29

## S1 – POWER CONSUMPTION OF ROBOTS AND BATTERY CHARACTERIZATION

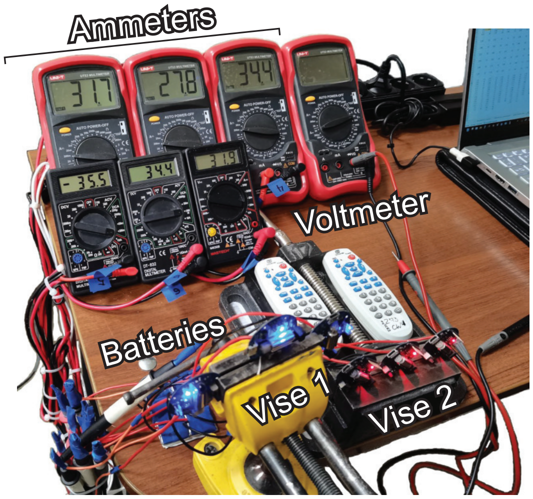


Figure S1: Experimental setup for discharging curves measurement. The setup includes three UT-53 and three DT-831 miltimeters working as ammeters (labeled as Ammeters), one UT-53 multimeter working as a voltmeter (labeled as Voltmeter), and two vises (Vise 1 and Vise 2) that fasten six Swarmodroid boards supplied with extended wires. The batteries (labeled Batteries) are fastened separately onto the table.

To evaluate the maximum continuous operation time of the Swarmodroid, we perform experimental measurements of battery discharge curves for six randomly selected bots. Prior to the measurement, each printed circuit board (PCB) is extracted from the plastic body and fixed in a vise. To prevent the wires connecting the PCB and the battery from falling apart due to vibration, the batteries are fastened onto the table using a double-sided adhesive tape (see Fig. S1), and the 2 cm long wires that connect the PCB to the battery are extended by $10 - 30$ cm. The bots firmware is alternated in a way that allows them continue vibrating even when the battery is discharged to the critical level of 3.3 V. The batteries are charged before the start of experiment until the charge current falls below 30 mA.

After charging, a voltmeter an ammeter are attached in parallel and in series to the battery, respectively. To measure the current, we connect UNI-T UT-53 and Mastech DT-831 multimeters in the ammeter mode ($0 - 200$ mA range) in series between the positive battery output and the PCB. The voltage is measured periodically by connecting UT-53 multimeter in the voltmeter mode ($0 - 20$ VDC range) between the positive and negative outputs of each battery.

The values of voltages and currents are measured every 30 minutes for PCBs vibrating at PWM = 10% and PWM = 30%, and every 20 minutes in the case of PWM = 50%. The moment of total discharge is defined as a time when the voltage level reaches 2.4 V. The obtained results are shown in Fig. S2. It is seen that the discharge time monotonically depends on the PWM level. However, the dependence in nonlinear: discharge times for PWM = 10% [Fig. S2(a,d)] are approximately two times higher than for PWM = 20% [Fig. S2(b,e)], while the difference between PWM = 10% and PWM = 30% [Fig. S2(c,f)] is about 25%, highlighting that a collector engine needs more current on low rotation frequencies. Despite the incremental reduction of measured characteristics (caused by a simultaneous decrease in voltage and current), the robots were able to exhibit stable motility during the major part of working time. Average working times are 10 h 11 m, 5 h 11 m, and 3 h 45 m for PWM = 10%, 20%, and 30%, respectively.

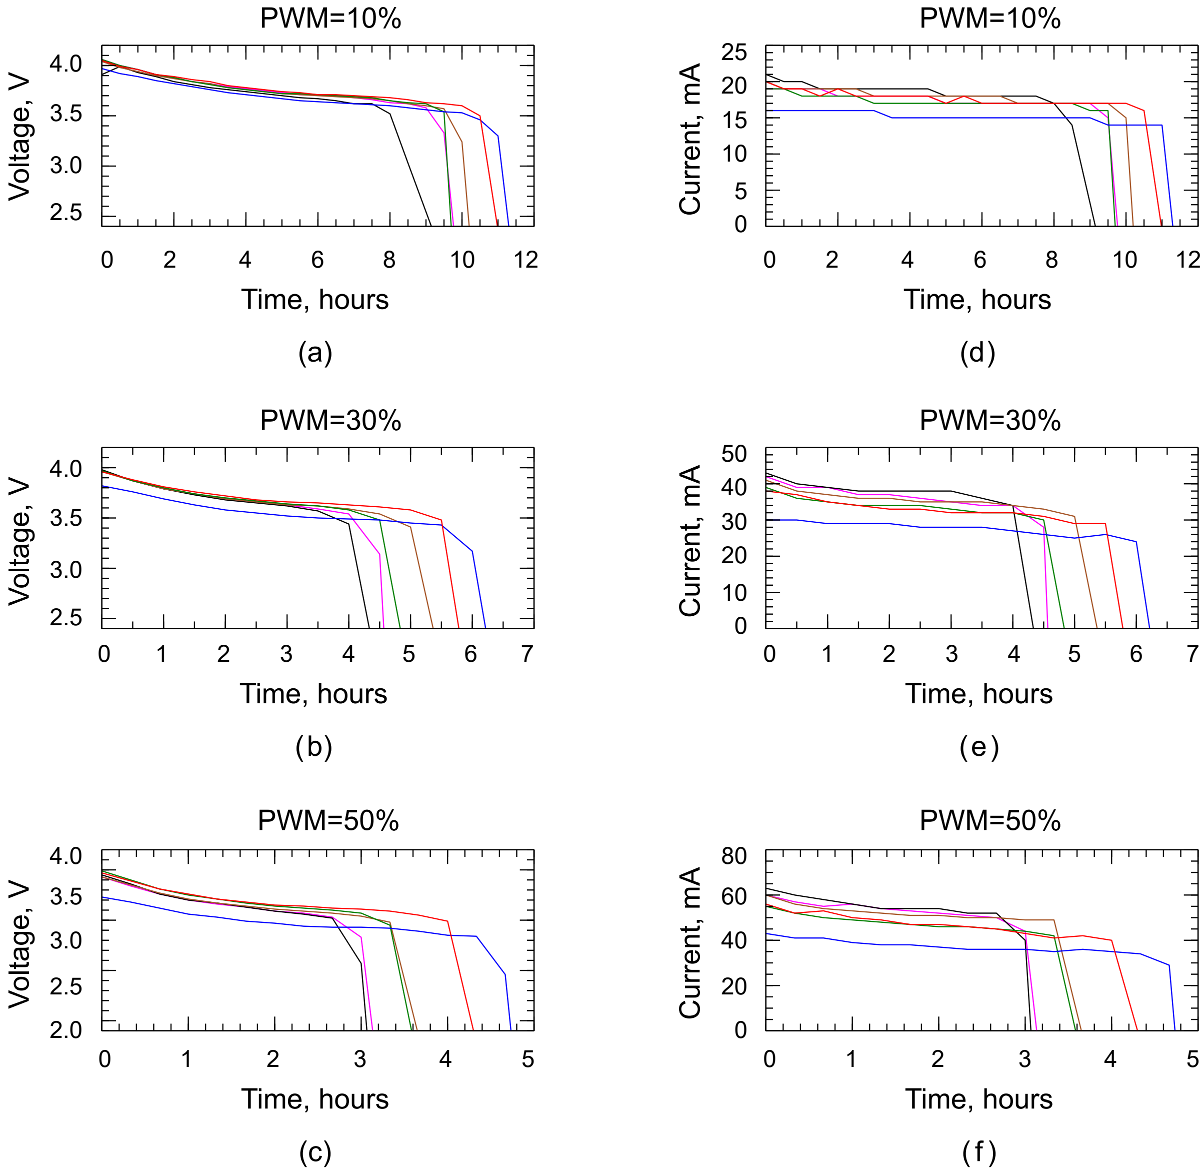


Figure S2: The measurements of the battery voltage (a-c) and current (d-f) for six Swarmodroid circuit boards working at the PWM rates 10%, 30%, and 50%, as specified in the respective panels. Different colors correspond to six different circuit boards. The matching of color to the board is the same throughout the panels.

## S2 – ALGORITHM OF THE ROBOT FIRMWARE

This section offers a simplified, but complete description of the algorithm that the MCU firmware follows. For comments concerning the implementation of this algorithm on an ATTiny13 unit, see Sec. S3

To describe the MCU firmware[1], let us divide it into into the following three parts: the `main` procedure, the 8-bit Timer/Counter and the interrupt service routines (ISR) that it executes, and the pin change interrupt ISR.

### S2.1 – The `main` procedure

The `main` procedure is executed at the moment the MCU is powered on, and follows the flowchart shown in Fig. S3. After initialization of the analog-digital converter (ADC), a self-test is performed to make sure that the battery voltage is above the critical level (approximately 3.3 V). First, the battery voltage level is measured with the motor powered off. The measured battery idle voltage is indicated by blinking the LED (`D1`) one time for a low charge level, two times for a medium level, and three times for a full charge, respectively. If it is below the critical level, the rest of the startup sequence is skipped.

As the next step of the startup sequence, a variable is allocated to store the previous reading of the 8-bit Timer/Counter; pin-change interrupt is enabled; the 8-bit Timer/Counter is set to free-run mode and started, enabling the PWM and IR remote control receive. After that, the PWM gate output is set to high for 50 ms, making the motor run at full power. A battery level measurement is performed at the same time to ensure the battery level at full load does not fall below the critical level. Finally, Timer/Counter overflow interrupt is enabled, and the corresponding ISR is set to perform a battery level measurement; the device waits for one second, enables global interrupts and lits up the LED to indicate the end of the startup sequence.

Now the device enters an infinite loop, which checks the battery voltage every second and does nothing else. All bot functionality is now performed by the interrupt service routines. If the battery level falls down to the critical level, the loop breaks and the bot enters the power-saving mode.

Upon entering this mode, the PWM output is forced constant low, the LED is turned off and all interrupts are globally disabled to make the bot unresponsive to any commands. After that, the LED is turned off and blinked briefly every three seconds to indicate that the bot needs to be charged.

[1] https://github.com/swarmtronics/swarmodroid.firmware

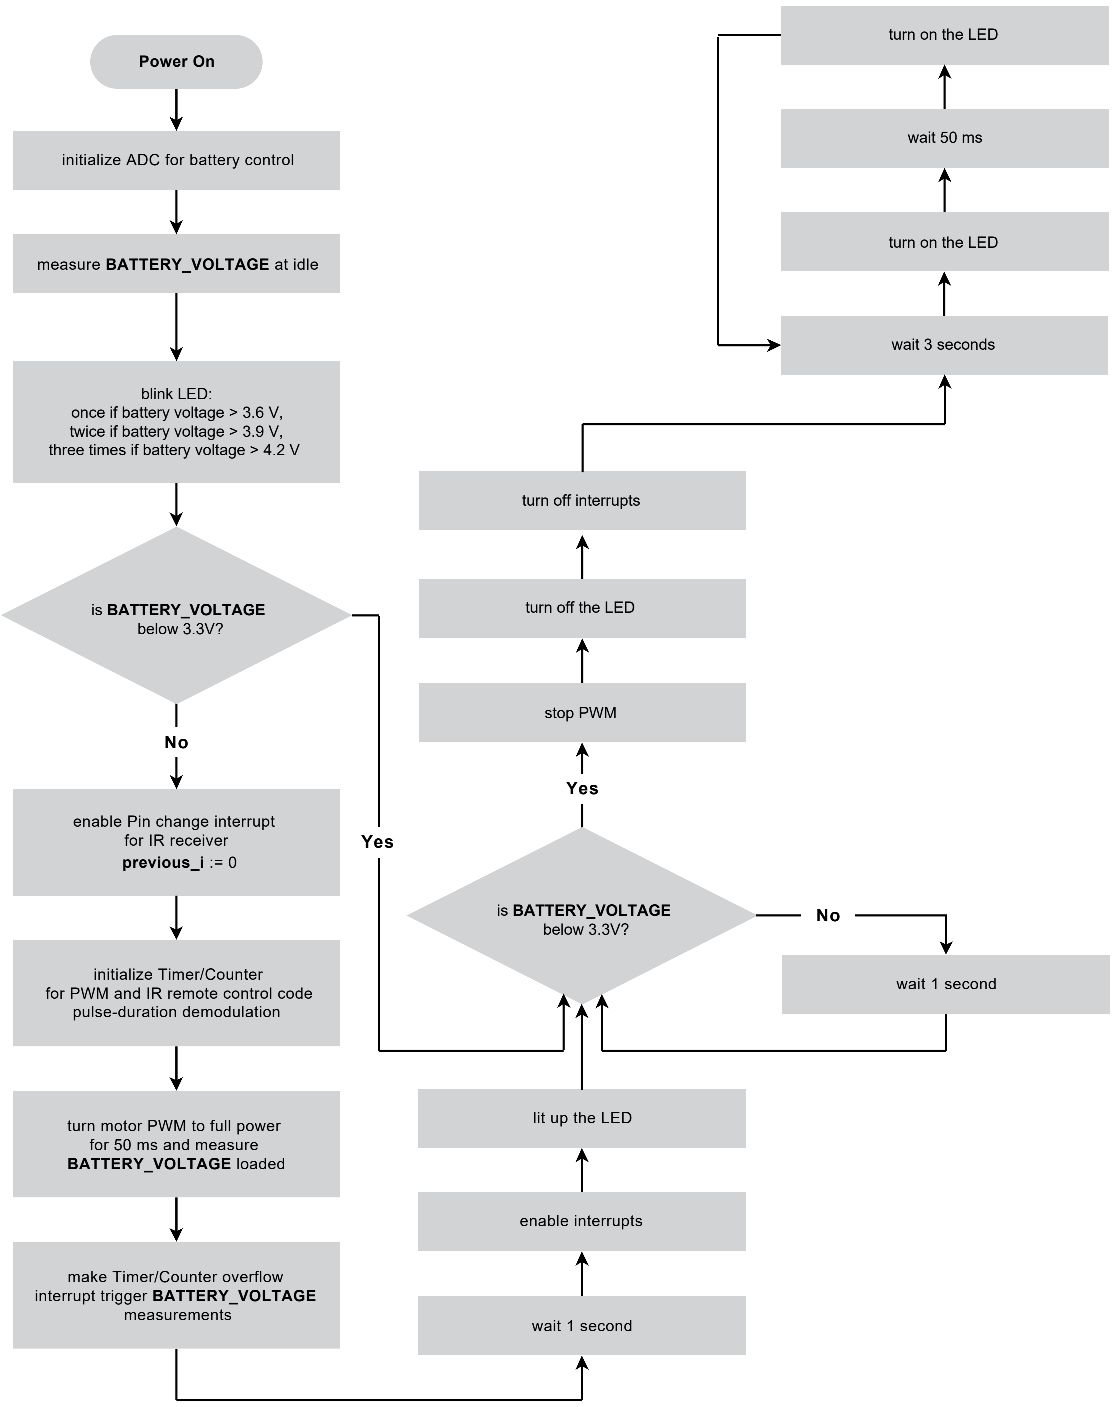


Figure S3: Flowchart of the bot firmware `main` procedure.

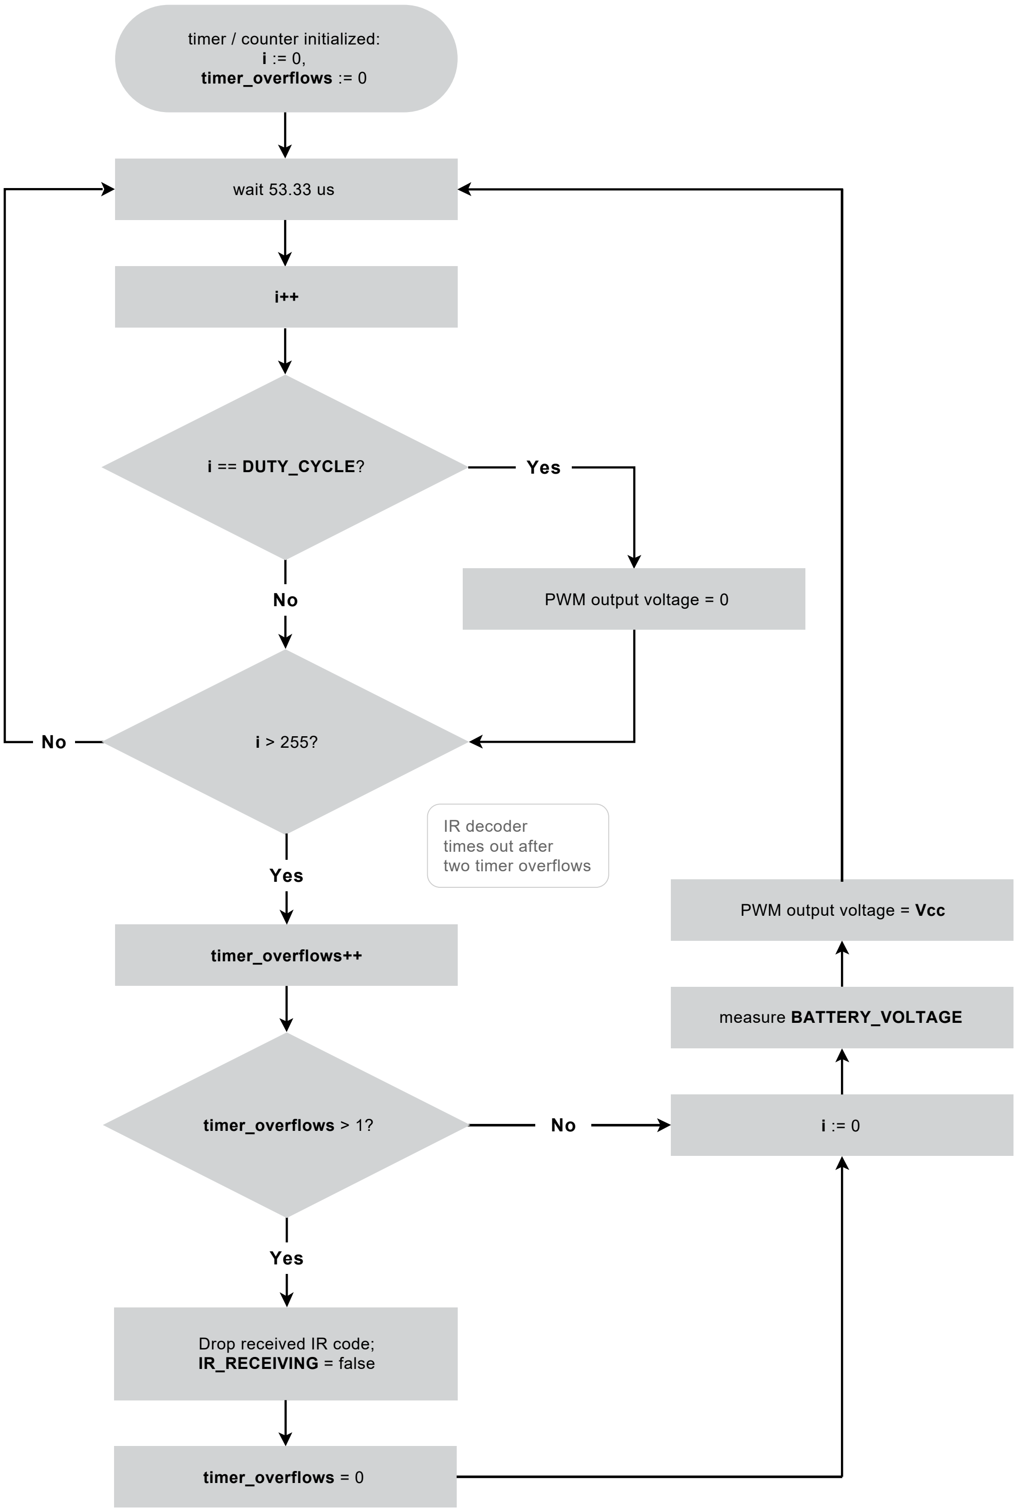


Figure S4: Flowchart of the bot firmware 8-bit Timer/Counter.

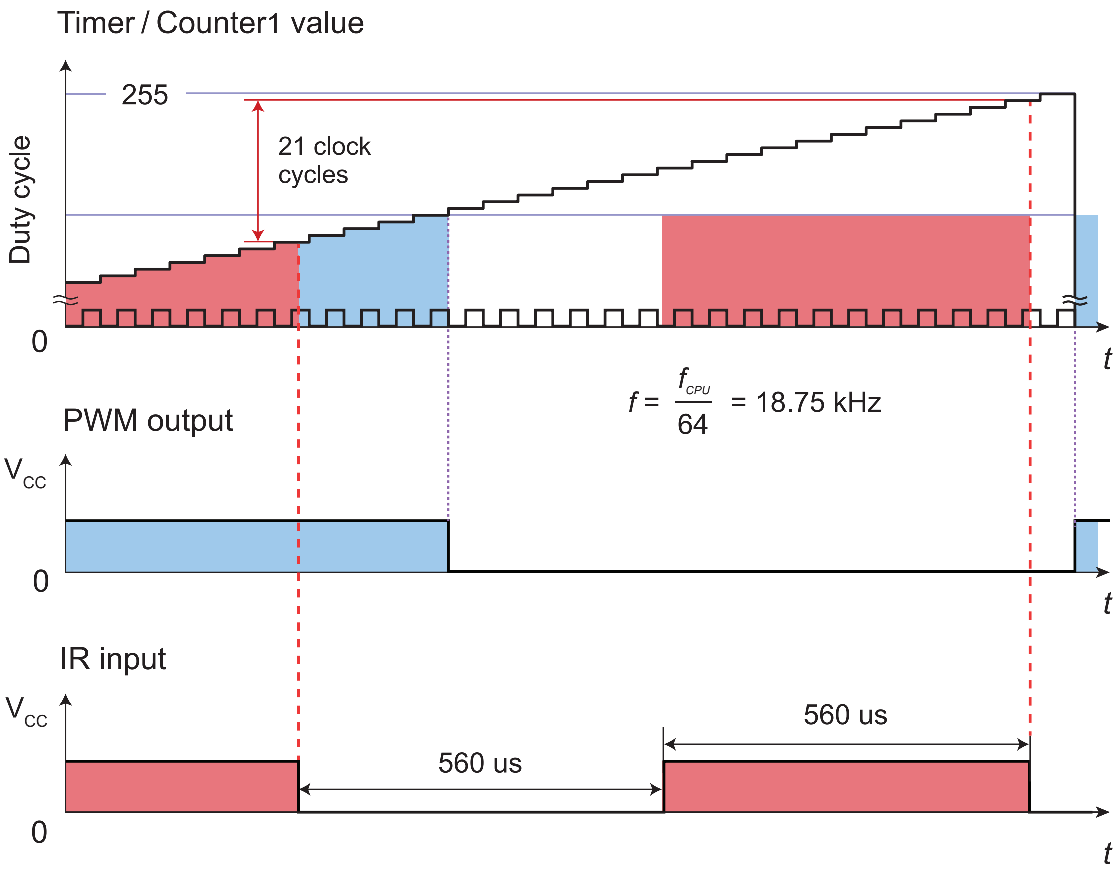


Figure S5: Timing diagram of the bot microcontroller unit.

**S2.2 – 8-bit Timer/Counter**

The microcontroller runs at the frequency $f_{\mathrm{CPU}} = 1.2$ MHz (9.6 MHz from internal RC oscillator divided by 8 by the CKDIV8 prescaler, as defined by the FUSEs ATTiny13A is shipped with). The Timer/Counter1 runs with a frequency equal to $f_{\mathrm{CPU}}/64$, as defined by the software-programmed prescaler setting – i.e., at $f = 18.75$ kHz. Each 53.3 µs the 8-bit Timer/Counter value is incremented.

While the main loop is running, the Timer/Counter is used simultaneously to generate the PWM signal, measure the pulse widths to demodulate the signal from the IR receiver, and to trigger periodic battery voltage checks. Its functionality can be demonstrated by a flowchart shown in Fig. S4. The timing diagram of the Timer/Counter is shown in Fig. S5.

*S2.2.0a – PWM signal generation* This Timer/Counter1 value is used to drive the PWM signal for the motor. Before starting the PWM, the 8-bit duty cycle is programmed. The PWM is then made to free-run. When the Timer/Counter1 value overflows, the PWM output is set to high. When the Timer/Counter1 value becomes equal to the programmed duty cycle value, the PWM output is set to low. Therefore, the PWM frequency is $f_{\mathrm{CPU}}/64/256 \simeq$ 73 Hz with 256 possible duty cycle values.

*S2.2.0b – Periodic battery level checks* At the Timer/Counter1 overflow event, a measurement of the loaded battery voltage using the ADC is triggered right after setting the PWM output to high. The resulting value is checked in the main loop.

*S2.2.0c – Pulse-period demodulation* The demodulation is mostly performed in the pin change interrupt ISR, described in detail in Sec. S2.3. The Timer/Counter carries two functions for the demodulation. First, the Timer/Counter's value is used for time measurement. To measure the time interval between two incoming falling pulse edges, the difference with its previous value, stored into a variable, is calculater in the pin change interrupt ISR.

The second function is the overflow counter. There is no pulse sequence in the NEC protocol, that is longer than $256 \times 53.3$ µs. Therefore, to avoid locking the pulse-period demodulation state machine locking in the "receiving 32 data bits" state if the transmission is aborted before 32 bits has been received, an automatic reset is needed if too

much time has passed since the last pulse edge. The second Timer/Counter1 overflow is used as the definition of "too much time", as the measurement by calculating the difference becomes meaningless anyway if more than one overflow has occurred.

To achieve that, an overflow counter is used. It is incremented at overflow events and reset to zero in the pin change interrupt service routine. Therefore, the overflow counter contains the number of Timer/Counter1 overflows since the last measurement. At Timer/Counter1 overflow event, the overflow counter is incremented. If, after the increment, the overflow counter reaches two, the state machine is reset from the "receiving 32 data bits" state to the "receiving not initiated" state.

### S2.3 – Pin change interrupt ISR

The NEC infrared transmission protocol uses the pulse-period modulation: after the initial pulse sequence, 32 bits of data are transmitted, encoded as (560 µs↓ + 560 µs↑) pulse pair for logical 0 and (560 µs↓ + 1680 µs↑) for logical 1 (here ↑ indicates 3.3 V level and ↓ indicates 0 V). The decoding is performed by measuring the distances between the falling pulse edges using Timer/Counter1 and processing them using a finite state automaton (FSA).

A pin-change interrupt is enabled on the pin that is connected to the infrared receiver output, so that an interrupt event is generated at each change of the logical level. At each pin change interrupt event, the corresponding interrupt service routine is executed and performes the actions shown by the flowchart in Fig. S6 to alter the state of the FSA according to the meaning of the received pulse.

First, the sign of the edge that caused the interrupt, is checked. Rising edges are ignored, except for the 4.5 ms↑ leading pulse (the lengths of the positive and negative pulses are measured separately in this case). If the interrupt was caused by a falling edge, the Timer/Counter1 value is stored to the `previous_TCNT1` variable. By calculating the difference between the current Timer/Counter1 value and the `previous_TCNT1` (overflow is permitted at this point), the pulse period (the distance between the falling edges) is measured within ±50 µs accuracy. In the NEC IR protocol, all meaningful pulse widths are multiples of 560 µs – up to the longest (9 ms↓ + 4.5 ms↑) pulse pair, which is approximately $253 \times 53.3$ µs. Therefore, such a measurement allows to discriminate between all pulse pairs occurring in the NEC protocol.

After the length of the positive-negative pulse pair has been measured, its meaning is analyzed. If it was a transmission-initiating sequence (9 ms↓ + 4.5 ms↑), then the FSA is put into the *receiving* state, and the shift register, which will hold the received value, is cleared.

If a pulse pair other than the transmission-initiating sequence has been received when the FSA is in the *non-receiving* state, it is ignored.

If the received pulse pair corresponds to either logical 0 (560 µs↓ + 560 µs↑) or logical 1 (560 µs↓ + 1680 µs↑) while the FSA is in the *receiving* state, the corresponding bit is shifted into the shift register. The shift register is then checked whether it contains all 32 bits. If not, nothing else is done. If all 32 bits have been received, the FSA is put to the *non-receiving* state, and the received bits are processed in the following way. The first (most-significant) 16 bits are compared to the hard-coded 16-bit address constant of the bot. If those are not equal, the command is understood as directed to some other device and is ignored. Next, the command, which is contained in the third byte, is checked for being valid by comparing it to the logical inverse of the fourth byte. If those are equal, the command is valid. It is then searched in the list of known commands, and, if found, the corresponding PWM duty cycle is chosen. In case the corresponding duty cycle is zero, the PWM output is driven to constant zero, and an indication of the battery voltage is performed.

If any other pulse pair is received in the *receiving* state, the entire pulse sequence is dropped and the FSA is reset into the *non-receiving* state.

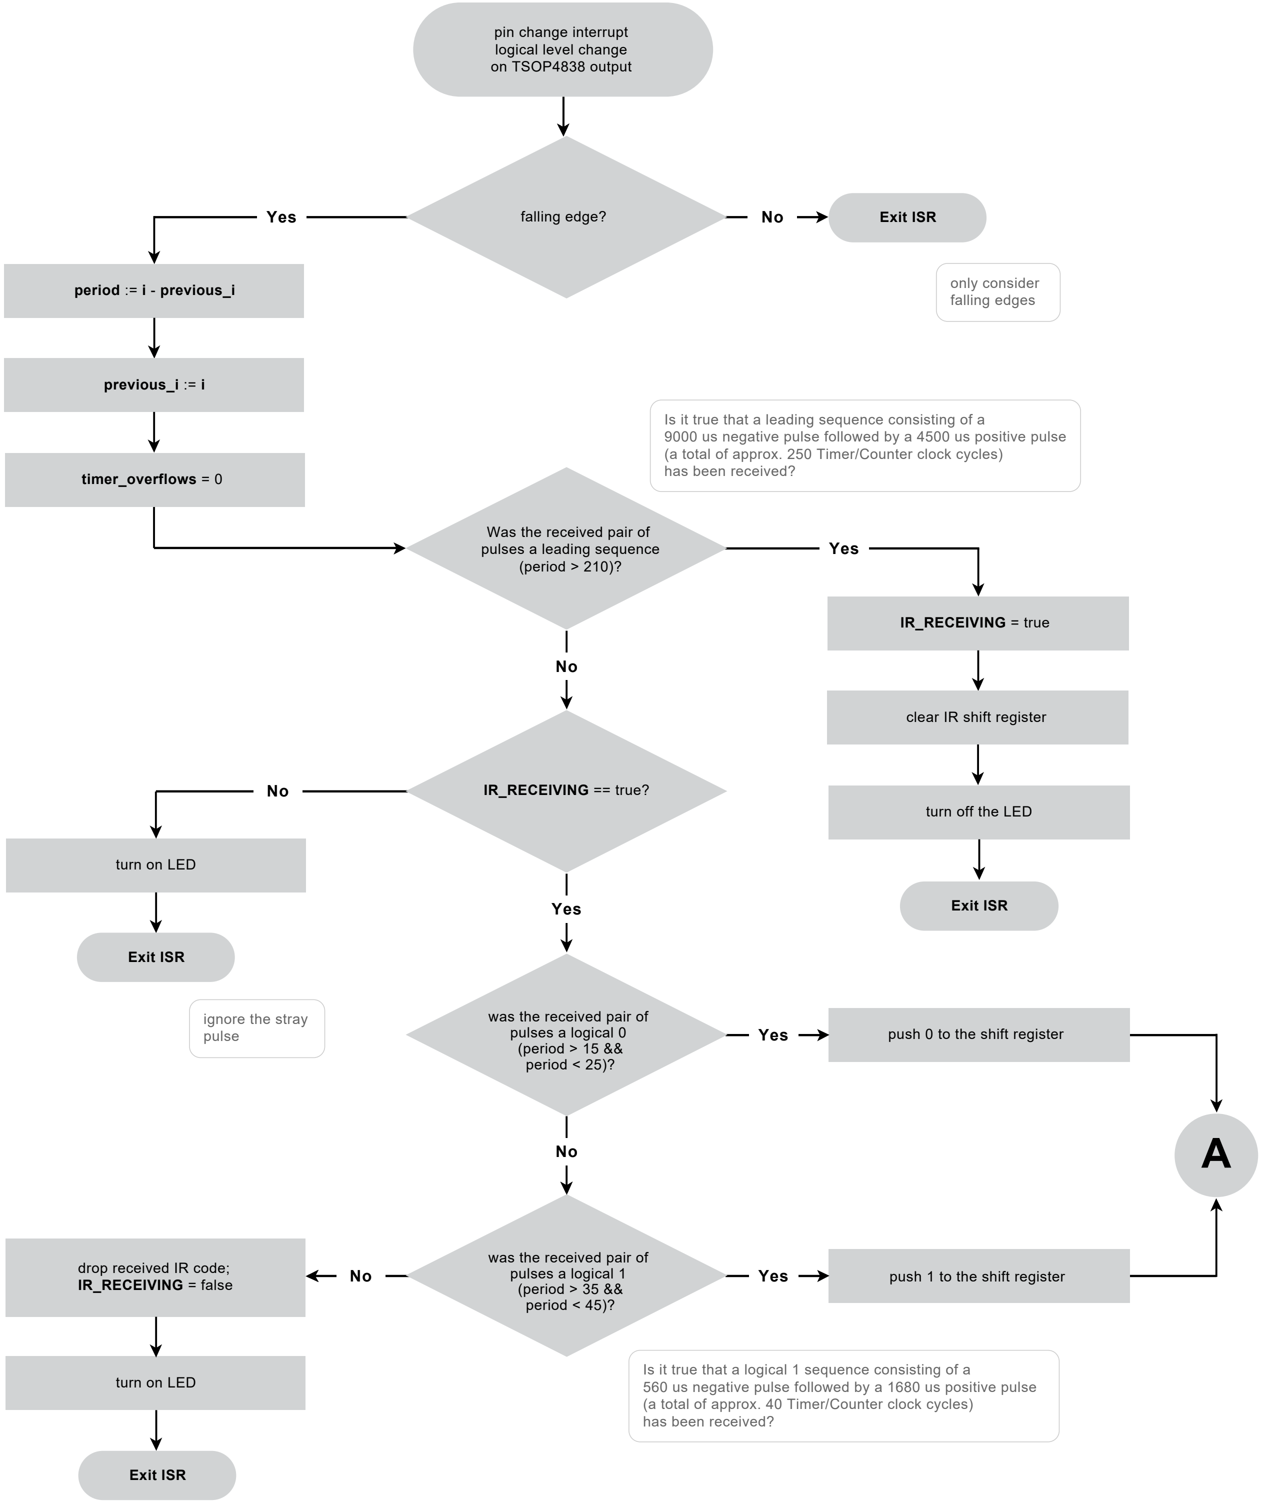


Figure S6: Flowchart of the bot firmware interrupt service routine (ISR) executed at pin change interrupt events.

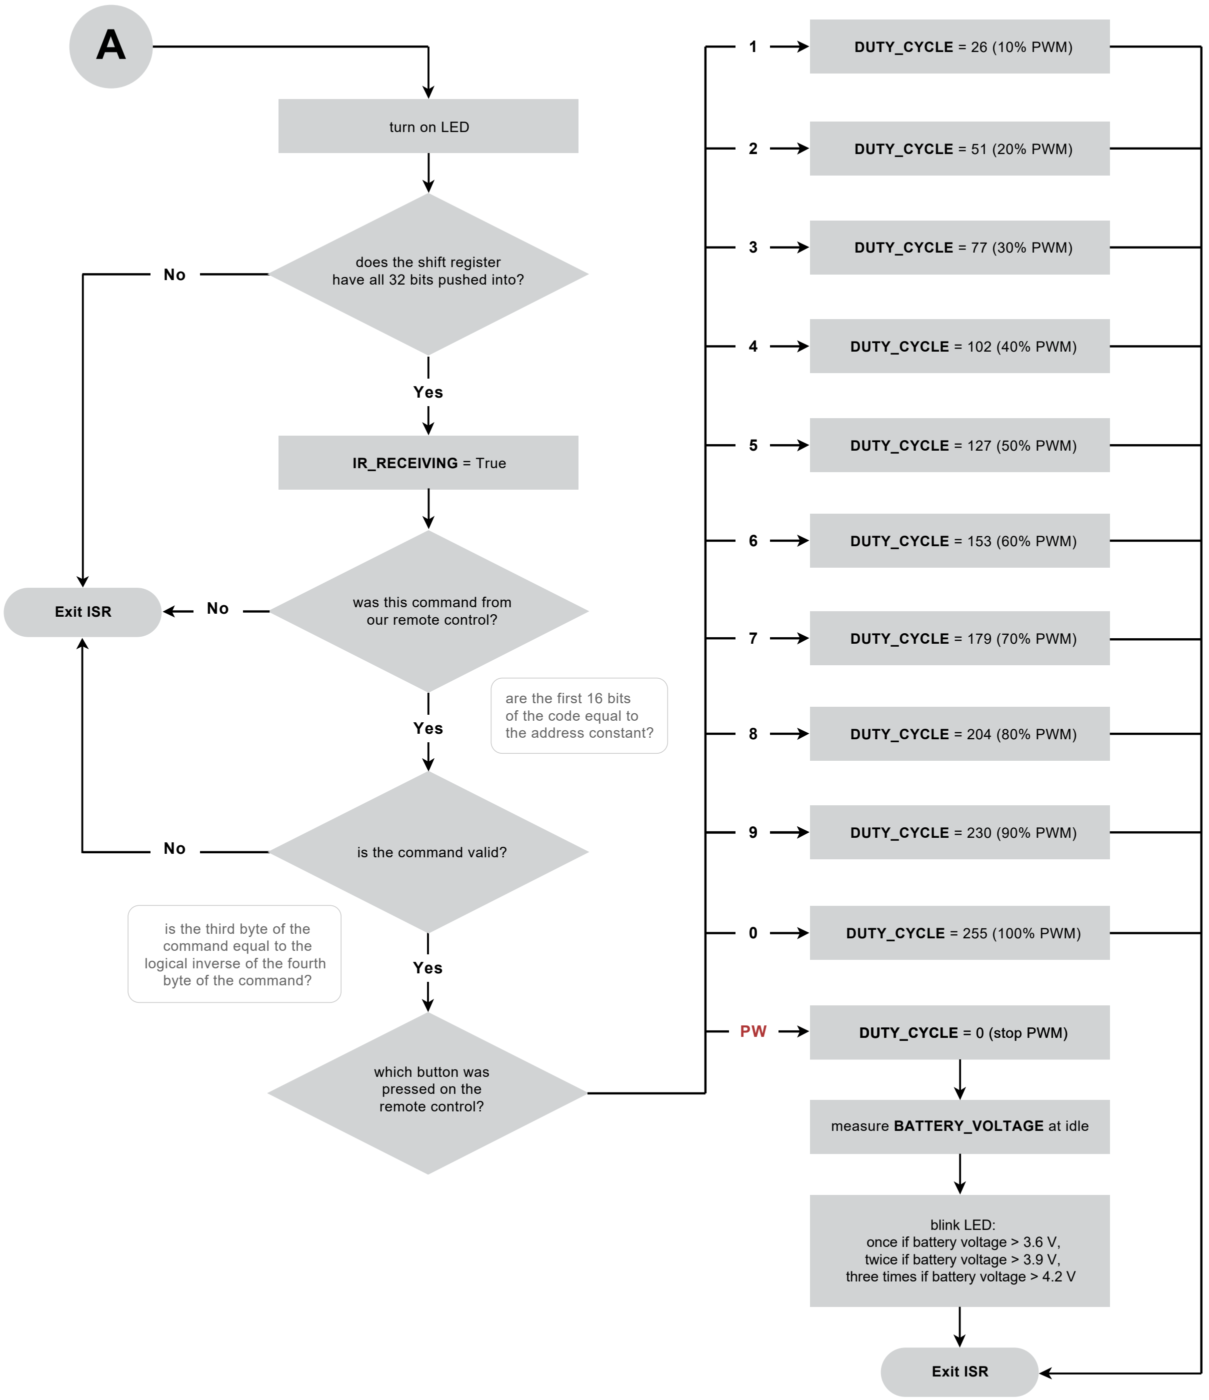


Figure S6 (continued): Flowchart of the bot firmware interrupt service routine (ISR) executed at pin change interrupt events.

## S3 – FIRMWARE REFERENCE

Here, a detailed description of each code block of the firmware is provided. Firmware is originally written in the C programming language, using the `avr-libc` library and is verified to compile correctly with avr-gcc 5.4.0 with the following options:

```
avr-gcc -mmcu=attiny13 -O2 -fshort-enums main.c
```

Note that the assembler code listed in this document has been partially changed to increase readability, and, while it performs the same actions, it does not correspond exactly to the object file produced by avr-gcc.

### S3.1 – Global variables

As the firmware relies heavily on the interrupts, it utilizes global volatile variables allocated in the heap, along with the registers. The following global variables are defined.

*S3.1.0a – State of the IR demodulator FSA*

**C code**

```c
typedef enum {
  IR_STATE_IDLE,
  IR_STATE_LEADING_9000ms,
  IR_STATE_LEADING_4500ms,
  IR_STATE_DATA_BITS
} ir_state_t;

volatile ir_state_t ir_state = IR_STATE_IDLE;
```

**Assembler code**

```
/* .section .bss */
.global  ir_state
  .type  ir_state, @object
  .size  ir_state, 1
ir_state:
  .zero  1

.equ IR_STATE_IDLE, 0
.equ IR_STATE_LEADING_9000ms, 1
.equ IR_STATE_LEADING_4500ms, 2
.equ IR_STATE_DATA_BITS, 3
```

The global variable `ir_state` holds the current state of the IR pulse-period demodulator state machine. The following states are possible:

0. `IR_STATE_IDLE` – the IR receiver output is held constantly at $V_{CC}$. The bot is waiting for a falling edge that initiates an incoming transmission. This is the default state.

1. `IR_STATE_LEADING_9000ms` – an incoming transmission falling edge has been encountered, a 9 ms logical low leading pulse now being received – the bot is now waiting for a rising edge.

2. `IR_STATE_LEADING_4500ms` – a 9 ms logical low leading pulse has been completely received, now a 4.5 ms logical high leading pulse is being received –the bot is now waiting for a falling edge.

3. `IR_STATE_DATA_BITS` – the 32 data bits are now being received. At this state, only full periods (falling edge to falling edge) are measured, so the timer is only read on falling edges. Rising edges are ignored at this state. When all 32 bits are successfully received, the FSA will be reset to `IR_STATE_IDLE`. The same will happen if an unexpected pulse sequence is encountered, with the only exception of a leading 9 ms pulse – in that case, the FSA is put back at `IR_STATE_LEADING_9000ms`.

*S3.1.0b – IR shift register*

**C code**

```c
uint32_t ir_shift_register = 0;
volatile uint8_t ir_received_bits_count = 0;
```

**Assembler code**

```
/* .section .bss */
.global  ir_shift_register
  .type  ir_shift_register, @object
  .size  ir_shift_register, 4
ir_shift_register:
  .zero  4
.global  ir_received_bits_count
  .type  ir_received_bits_count, @object
  .size  ir_received_bits_count, 1
ir_received_bits_count:
  .zero  1
```

The global variable `ir_shift_register` is a 32-bit shift register that incoming IR 32-bit pulse sequences are clocked into. `ir_received_bits_count` is a counter that is used to stop receiving bits when all 32 bits are received, and which is also reset to zero to drop any bit sequences that have not been completely received due to a timeout or a malformed pulse sequence.

*S3.1.0c – Timer/Counter previous value*

**C code**

```c
volatile uint8_t previous_TCNT0_value = 0;
volatile uint8_t timer_overflow_flag;
```

**Assembler code**

```
/* .section .text */
.comm  timer_overflow_flag,1,1

/* .section .bss */
.global  previous_TCNT0_value
  .type  previous_TCNT0_value, @object
  .size  previous_TCNT0_value, 1
previous_TCNT0_value:
  .zero  1
```

The global variable `previous_TCNT0_value` holds the previous value of the 8-bit Timer/Counter. The current value is stored by the timer in the register `TCNT0`. The global flag variable `timer_overflow_flag` is a 1-bit overflow counter, which indicates a non-zero count of Timer/Counter overflows happened since the last time `TCNT0` has been stored into `previous_TCNT0_value` using the macro `start_time_interval_measurement()` or `get_time_interval_since_last_measurement()`. If this flag is set, at a subsequent Timer/Counter overflow event, handled by the Timer/Counter overflow interrupt service routine, the received IR bits will be dropped due to a timeout. The reason is that we use the difference between the current timer/counter value and its previous value to measure the pulse widths. This allows correct measurement even if a timer overflow has happened once, but not twice. We therefore use the second overflow as a trigger to hang up the IR receive.

*S3.1.0d – Battery critical discharge flag*

**C code**

```c
volatile uint8_t battery_status_critical;
```

**Assembler code**

```
/* .section .text */
.comm  battery_status_critical,1,1
```

The global flag variable `battery_status_critical` indicates that the battery voltage has fallen down to a critical level. This variable is updated and read in an asynchronous manner. First, at a Timer/Counter overflow event, an ADC measurement is triggered by the auto-trigger function. As soon as the measurement is finished, the ADC measurement complete interrupt service routine updates the `battery_status_critical` variable by executing the macro `ensure_battery_level_above_critical()`. Finally, this flag is read each second in the main loop, which is terminated as soon as the flag is read as set.

## S3.2 – Macro definitions: hardware-related constants

*S3.2.0a – Time bases* First, we define the constants related to the MCU clock frequency.

**C code**

```c
#define F_CPU 1200000UL
#define F_CPU_ACCURACY_PERCENT 20
```

**Assembler code**

```
.equ F_CPU, 1200000
.equ F_CPU_ACCURACY_PERCENT, 20
```

The constant `F_CPU` is defined to be equal to the MCU clock frequency in Hz, as a 4-bit unsigned integer number. In our case, the MCU runs at factory fuses: 9.6 MHz frequency with `CKDIV8` (divide the clock frequency by 8) enabled, therefore the CPU is clocked at 1.2 MHz. This constant is used as a general time base for milliseconds to clock cycles conversion to create delays and for microseconds to Timer/Couter ticks conversion for pulse-period demodulation of the IR signals.

The constant `F_CPU_ACCURACY_PERCENT` is defined to simplify the conversion from the number of Timer/Counter cycles to the actual time in microseconds using macros. We assume the 20% accuracy of the CPU frequency, as the MCU is clocked using its internal RC oscillator, which we do not calibrate.

**C code**

```c
#define TCNT_PRESCALER  64
```

**Assembler code**

```
.equ TCNT_PRESCALER, 64
```

This macro carries the value of the Timer/Counter prescaler. We set the Timer/Counter to run at $f = F_{\mathrm{CPU}}/64 =$ 18.75 kHz.

*S3.2.0b – Pin function constants*

**C code**

```c
#define BIT_PWM 1
#define BIT_LED 2
#define BIT_IR 3
#define BIT_ADC 4
```

**Assembler code**

```
.equ BIT_PWM, 1
.equ BIT_LED, 2
.equ BIT_IR, 3
.equ BIT_ADC, 4
```

These macros match the bits of `PORTB` and the corresponding electronic components (MOSFET gate, LED, output of the IR receiver and the voltage divider for battery level measurements, respectively) on the actual printed circuit board. Note that the PWM pin doubles as `OCR0B` (the Timer/Counter PWM output).

*S3.2.0c – Battery charge levels*

**C code**

```c
#define BATTERY_CRITICAL        131
#define BATTERY_LEVEL_SPACING   12
```

**Assembler code**

```
.equ BATTERY_CRITICAL, 131
.equ BATTERY_LEVEL_SPACING, 12
```

The first macro holds the `ADCH` reading (the most-significant byte of the ADC reading, while the value is left-adjusted) corresponding to the critical battery level. The second value holds the spacing between the battery levels, in `ADCH` reading units. These constants are obtained as follows. The ADC is multiplexed to the pin, which is connected to $V_{\mathrm{CC}}$ through a $R_1 : R_2$ resistor voltage divider. Therefore, the 10-bit ADC reading equals

$$\mathrm{ADC} = 1024 \cdot \frac{V_{\mathrm{CC}}}{V_{\mathrm{ref}}} \frac{R1}{R1 + R2},$$

where $R_1 = 680\ \Omega$ and $R_2 = 3300\ \Omega$ are the values of the resistors in the voltage divider, and $V_{\mathrm{ref}} = 1.1$ V is the voltage provided by the MCU built-in bandgap reference. We configure the ADC for left-aligned 10-bit-in-uint16 storage, therefore

```
ADCW = ADC << 6 (16-bit value),
```

`ADCH = (ADCW >> 2) & 0xFF.`

The ADC and `ADCH` readings corresponding to each of the four defined battery levels is, therefore, defined according to Table S1, and the spacing between the levels is 12.

| Battery level | $V_{CC}$ | ADC reading (decimal) | `ADCH` reading (decimal) |
|---|---|---|---|
| critical | 3.3 V | 524 | 131 |
| low | 3.6 V | 572 | 143 |
| medium | 3.9 V | 620 | 155 |
| full | 4.2 V | 668 | 167 |

Table S1: Battery levels indicated by the Swarmodroid and the corresponding ADC readings.

*S3.2.0d – ADC multiplexer helper macros*

**C code**

```
#define ADC_ON_PB2 1
#define ADC_ON_PB3 3
#define ADC_ON_PB4 2
#define ADC_ON_PB5 0
```

**Assembler code**

```
.equ ADC_ON_PB2, 1
.equ ADC_ON_PB3, 3
.equ ADC_ON_PB4, 2
.equ ADC_ON_PB5, 0
```

Finally, we define ADC multiplexer constants, to select the pin the ADC will be listening to. Refer to the description of the `ADCMUX` register in the ATTiny13A documentation [1].

### S3.3 – Macro definitions: inline functions

*S3.3.0a – Delay loops* The firmware relies on empty loops to create delays. In the C code, the utility macros defined in `util/delay.h` are used. In assembly code, we define our own macros for delay creation.

**C code**

```
#include <avr/interrupt.h>
#include <util/delay.h>
```

In C code, the headers `avr/interrupt.h` and `util/delay.h` containing macro definitions from the avr-libc are included. For `util/delay.h` to work properly, the constant `F_CPU` must be defined prior to inclusion of `util/delay.h` and set to correspond to the actual clock frequency of the device.

In assembler code, one may define the following two macros to substitute those defined in `util/delay.h`. As in the C code, the constant `F_CPU` must be defined earlier.

**Assembler code**

```
.macro delay16bit_r24_r25 delay_ms
  .set DELAY, (F_CPU / 4000 * delay_ms - 1)
  ldi r24, lo8(DELAY)
  ldi r25, hi8(DELAY)
  1: sbiw r24, 1
  brne 1b
  rjmp .
  nop
.endm
```

**Assembler code**

```
.macro delay24bit delay_ms reg1 reg2 reg3
    .set DELAY, (F_CPU / 5000 * delay_ms - 1)
    ldi \reg1,lo8(DELAY)
    ldi \reg2,hi8(DELAY)
    ldi \reg3,hlo8(DELAY)
    1:
    subi \reg1,1
    sbci \reg2,0
    sbci \reg3,0
    brne 1b
    rjmp .
    nop
.endm
```

*S3.3.0b – LED signalling* The following macros, defined for code readability, correspond to switching the LED on and off.

**C code**

```
#define led_on() { \
  PORTB |= 1 << BIT_LED; \
}
```

**Assembler code**

```
.macro led_on
    sbi PORTB, BIT_LED
.endm
```

**C code**

```
#define led_off() { \
  PORTB &= ~(1 << BIT_LED); \
}
```

**Assembler code**

```
.macro led_off
    cbi PORTB, BIT_LED
.endm
```

*S3.3.0c – PWM on/off*

**C code**

```
#define pwm_start() { \
  PORTB |= (1 << BIT_PWM); \
  DDRB |= (1 << BIT_PWM); \
}

```

**Assembler code**

```
.macro pwm_start
    sbi PORTB, BIT_PWM
    sbi DDRB, BIT_PWM
.endm
```

This macro enables the PWM by unlocking the write operations to the corresponding pin of `PORTB`, and puts the PWM output to logical high.

**C code**

```
#define pwm_stop() { \
  PORTB &= ~(1 << BIT_PWM); \
  DDRB &= ~(1 << BIT_PWM); \
}
```

**Assembler code**

```
.macro pwm_stop
    cbi PORTB, BIT_PWM
    cbi DDRB, BIT_PWM
.endm
```

This macro forces the PWM output to logical low and locks the corresponding pin of `PORTB` for write operations, thus force switching the PWM off.

*S3.3.0d – IR hangup*

**C code**

```
#define ir_hangup() { \
  ir_state = IR_STATE_IDLE; \
  led_on(); \
}
```

**Assembler code**

```
.macro ir_hangup
  sts ir_state,__zero_reg__
  led_on
.endm
```

This macro is used to drop the IR received bits. The FSA is reverted to the non-receiving (idle) state, and the LED is switched back on.

*S3.3.0e – Time interval measurement*

**C code**

```
#define start_time_interval_measurement() \
  previous_TCNT0_value = TCNT0; \
  timer_overflow_flag = 0
```

**Assembler code**

```
.macro start_time_interval_measurement reg
    in \reg, TCNT0
    sts previous_TCNT0_value, \reg
    sts timer_overflow_flag,__zero_reg__
.endm
```

This macro remembers the current Timer/Counter reading (`TCNT0`) into the global variable `previous_TCNT0_value` that stores its previous value. The timer overflow counter is also reset to zero.

**C code**

```
#define get_time_interval_since_last_measurement() \
  TCNT0 - previous_TCNT0_value; \
  start_time_interval_measurement()
```

**Assembler code**

```
.macro get_time_interval_since_last_measurement out reg
    in \out, TCNT0
    lds \reg, previous_TCNT0_value
    sub \out, \reg
    start_time_interval_measurement \reg
.endm
```

The second macro does the same as the first one, while also returning the time interval since the previous measurement.

*S3.3.0f – Setting PWM duty cycle*

**C code**

```
#define pwm_set_duty_cycle(duty_cycle) { \
  OCR0B = duty_cycle; \
  if(duty_cycle){ \
    pwm_start(); \
  } else { \
    pwm_stop(); \
    measure_and_show_battery_idle_voltage(); \
  } \
}
```

**Assembler code**

```
.macro pwm_set_duty_cycle pwmreg exitlabel
    out OCR0B, \pwmreg
    tst \pwmreg
    breq 1f
    pwm_start
    rjmp \exitlabel
    1:
    pwm_stop
    rcall measure_and_show_battery_idle_voltage
    rjmp \exitlabel
 .endm
```

This macro updates the duty cycle register `OCR0B`, while treating the zero duty cycle case in a special manner. As the smallest duty cycle supported by the Timer/Counter PWM is 1/256, to avoid voltage spikes at zero duty cycle, the PWM output is explicitly forced low in this case. For convenient battery level checking, the battery voltage is

also indicated by LED blinking, if a zero duty cycle has been selected.

*S3.3.0g – Battery level measurement*

**C code**

```c
#define adc_fire_once(){ \
  ADCSRA |= (1 << ADSC); \
  loop_until_bit_is_set(ADCSRA, ADIF); \
}
```

**Assembler code**

```
.macro adc_fire_once
    sbi ADCSRA, ADSC
    1: sbis ADCSRA, ADIF
    rjmp 1b
.endm
```

Launch the ADC once and wait for it to finish in a synchronous manner. The 10-bit reading will be stored in the 16-bit register `ADCW`.

**C code**

```c
#define ensure_battery_level_above_critical() { \
  if (ADCH <= BATTERY_CRITICAL) { \
    pwm_stop(); \
    battery_status_critical = 1; \
  } \
}
```

**Assembler code**

```
.macro ensure_battery_level_above_critical reg
  in \reg, ADCH
  cpi \reg, (BATTERY_CRITICAL+1)
  brsh 1f
  cbi PORTB, BIT_PWM
  cbi DDRB, BIT_PWM
  ldi \reg, 1
  sts battery_status_critical, \reg
1:
.endm
```

This macro utilizes the value `ADCH` previously measured by the ADC (in an asynchronous manner), to make sure that the battery level has not fallen below critical. If it did, the PWM is immediately stopped, and the global flag variable `battery_status_critical`, which is watched by the main loop, is updated to break the main loop and enter the power-saving mode.

### S3.4 – Macro definitions: definitions introduced for code clarity

*S3.4.0a – Microseconds to Timer/Counter cycles conversion*

**C code**

```c
#define usec_to_cycles(time_us, error_percent) \
  (uint8_t) (F_CPU / 1000UL * (100 + (error_percent)) * (time_us) / TCNT_PRESCALER / 1000UL / 100)
```

**Assembler code**

```
.macro set_cycles_from_usec time_us, error_percent
    .set CYCLES_LO, (F_CPU / 1000 * (100 - \error_percent) * (\time_us) / TCNT_PRESCALER / 1000 / 100)
    .set CYCLES_HI, (F_CPU / 1000 * (100 + \error_percent) * (\time_us) / TCNT_PRESCALER / 1000 / 100)
.endm
```

This macro is used convert microseconds to Timer/Counter clock cycles (approx. 53.3 µs) at compile time, and is introduced for code readability: so that times are explicitly written in microseconds in code. As the CPU frequency, as well as the incoming pulse train frequency, might deviate significantly from the configured value, we introduce a second argument `error_percent`, which is the supposed deviation in an integer number of percents. This is used to compute intervals, given by the CPU frequency accuracy. The usage is to compare the time interval measured by the Timer/Counter to the expected time interval, for example:

**C code**

```c
uint8_t time_interval =
    get_time_interval_since_last_measurement();
if ((time_interval < usec_to_cycles(60, +20))
 && (time_interval > usec_to_cycles(60, -20)))
    puts("time interval is 60 microseconds +/- 20%");
```

**Assembler code**

```
get_time_interval_since_last_measurement r24 r25
set_cycles_from_usec 60, 20
ldi r25,lo8(-CYCLES_LO - 1)
add r25,r24
cpi r25,lo8(CYCLES_HI - CYCLES_LO - 1)
brsh .+2
rjmp time_interval_length_in_60usec_20percent_limits:
time_interval_length_out_of_60usec_20percent_limits:
```

*S3.4.0b – Function prologues and epilogues in assembler code* For concise representation of function prologues and epilogues in assembler code, i.e., the creation and removal of a stack frame, the following macros are introduced:

```
__SP_L__ = 0x3d
__SREG__ = 0x3f
__tmp_reg__ = 0
__zero_reg__ = 1

.macro push_status
    push r1
    push r0
    in r0,__SREG__
    push r0
    clr __zero_reg__
.endm

.macro pop_status
    pop r0
    out __SREG__,r0
    pop r0
    pop r1
.endm
```

The following macro `for_registers` is used to apply an operation sequentially to a given range of registers. The macros `for_register` and `eval_expr_and_for_register` are helpers used for correct expansion of arithmetic expressions.

```
.altmacro
.macro for_registers from, to, opcode
  for_register \from, \opcode
  .ifgt (to - from)
    for_registers (\from+1), \to, \opcode
  .endif
  .iflt (to - from)
    for_registers (\from-1), \to, \opcode
  .endif
.endm

.macro  for_register expr, opcode
  eval_expr_and_for_register %expr, \opcode
.endm

.macro  eval_expr_and_for_register number, opcode
```

```
  \opcode r\number\()
.endm
```

Namely, `for_registers, push, 17, 31` saves all user registers to the stack, while `for_registers, pop, 31, 17` retrieves them in a correct first-in-last-out order.

### S3.5 – Remote control constants

A separate header file `ir_remote_control_codes` defines a list of the known IR commands and the corresponding PWM duty cycles, in the form of a static array of structures, as well as the IR address.

**C code**

```c
#include "ir_remote_control_codes.h"
```

**Assembler code**

```
.include "ir_remote_control_codes.defs"
```

Let us review the contents of this file in detail. First, it defines the bot IR address.

**C code**

```c
#define REMOTECONTROL_ADDRESS 0x1CE3
```

**Assembler code**

```
.equ REMOTECONTROL_ADDRESS, 0x1CE3
```

The first 16 bits of all commands received from an IR remote control are first checked against this value, and if they are not equal, the command is ignored.

The second part of the `ir_remote_control_codes` file defines a list of IR command – PWM duty cycle pairs, 8 bit each. For clarity, these pairs are stored in a structure `ir_button_t`.

**C code**

```c
typedef struct {
  uint8_t command;
  uint8_t pwm_duty_cycle;
} ir_button_t;
```

**Assembler code**

```
.macro ir_button_t command, pwm_duty_cycle
  .byte \command
  .byte \pwm_duty_cycle
.endm
```

The values themselves are stored in a constant list of `ir_button_t`.

**C code**

```c
const ir_button_t IR_REMOTE_CONTROL_BUTTONS[] = {
  {
    .command = 0x48,
    .pwm_duty_cycle = 0
  },
  {
    .command = 0x80,
    .pwm_duty_cycle = 13
  },
}
```

**Assembler code**

```
.equ LIST_SIZE, 2
.global  IR_REMOTE_CONTROL_BUTTONS
  .section  .rodata
  .type  IR_REMOTE_CONTROL_BUTTONS, @object
  .size  IR_REMOTE_CONTROL_BUTTONS, (2 * LIST_SIZE)
IR_REMOTE_CONTROL_BUTTONS:
    ir_button_t 0x48, 0
    ir_button_t 0x80, 13
```

### S3.6 – `measure_and_show_battery_idle_voltage` function

This function measures the battery voltage in a synchronous manner and indicates it by blinking the signal LED several times: once for low level, twice for med, and three times for the high level, according to Table S1.

#### C code

```c
void measure_and_show_battery_idle_voltage() {
  adc_fire_once();
  int8_t battery_level = ADCH - (BATTERY_CRITICAL + BATTERY_LEVEL_SPACING);
  while(battery_level >= 0){
    led_on();
    _delay_ms(400);
    led_off();
    _delay_ms(400);
    battery_level -= BATTERY_LEVEL_SPACING;
  }
}
```

#### Assembler code

```asm
.equ SIGN_BIT, 7

.global measure_and_show_battery_idle_voltage
.type measure_and_show_battery_idle_voltage, @function
measure_and_show_battery_idle_voltage:
adc_fire_once
in r24, ADCH
subi r24, (BATTERY_CRITICAL + BATTERY_LEVEL_SPACING)
sbrc r24, SIGN_BIT
rjmp .LSHOW_BAT_VOLT_EPILOGUE
.LSHOW_BAT_VOLT_LOOP:
led_on
delay24bit 400 r18 r19 r25
led_off
delay24bit 400 r18 r19 r25
subi r24, BATTERY_LEVEL_SPACING
sbrs r24, SIGN_BIT
rjmp .LSHOW_BAT_VOLT_LOOP
.LSHOW_BAT_VOLT_EPILOGUE:
ret
.size measure_and_show_battery_idle_voltage, .-measure_and_show_battery_idle_voltage
```

The algorithm is as follows. First, the supply voltage is measured synchronously by executing the `adc_fire_once` macro. The higher byte `ADCH` of the measured value is then evaluated. The value is shifted relative to the critical level, as defined by the constant `BATTERY_CRITICAL`. After that, the LED is blinked for 800 ms corresponding to each battery level, while subtracting `BATTERY_LEVEL_SPACING` until the value becomes negative – the loop is terminated in this case.

### S3.7 – `main` function

The `main` function is executed at power-up, takes no arguments and returns no values (i.e., it has a prototype `void main(void)`) and is responsible for executing the startup sequence, running an infinite waiting loop, and, as

soon as the battery is discharged to the critical level, indication of the critical level by yet another infinite loop.

Next are the code blocks executed by the `main` function, given in the order of execution.

*S3.7.0a – ADC initialization* To initialize the ADC, the following bits are set in the ADC control registers.

ADC multiplexer control register (`ADMUX`):

- bit mask `ADC_ON_PB4` (2nd bit set only) – select the pin PB4 as the source of the analog signal;
- bit `REFS0` – select the internal 1.1 V bandgap reference as the source of the reference voltage;
- bit `ADLAR` – left-adjust the 10-bit conversion result in the 16-bit register `ADCW`.

ADC control register A (`ADCSRA`):

- bit `ADEN` – enable the Analog-Digital converter in the Single Conversion mode;
- bit mask `0x4` (3rd bit set only) – set the frequency to 1/16 of the CPU frequency (75 kHz) to ensure there is enough time for a 10-bit conversion (the ADC must not exceed 200 kHz for that).

After setting the control registers, the ADC is fired once to finish its initialization.

**C code**

```
ADMUX = ADC_ON_PB4 | (1 << REFS0) | (1 << ADLAR);
ADCSRA = (1 << ADEN) | 4;
adc_fire_once();
```

**Assembler code**

```
.global  main
  .type  main, @function
  .section  .text.startup,"ax",@progbits
main:
ldi r24, 0x62
out ADMUX, r24
ldi r24, 0x84
out ADCSRA, r24
adc_fire_once
```

*S3.7.0b – Initial battery level check* At the initial battery level check, first, the write operations are allowed by setting the second bit of `DDRB` to enable the LED indication. Then the global variable `battery_status_critical` is initialized to zero. The function `measure_and_show_battery_idle_voltage()` is then called to indicate the battery voltage level at idle by blinking the LED. At last, the battery level is ensured to be above critical, and in case it is not, the rest of the startup sequence is skipped.

**C code**

```
DDRB |= 1 << BIT_LED;
battery_status_critical = 0;
measure_and_show_battery_idle_voltage();
ensure_battery_level_above_critical();
```

**Assembler code**

```
sbi DDRB, BIT_LED
sts battery_status_critical, __zero_reg__
rcall measure_and_show_battery_idle_voltage
ensure_battery_level_above_critical r24
```

*S3.7.0c – Second part of the startup sequence* In the second part of the startup sequence, the following register bits are set.

Global interrupt mask (`GIMSK`):

- bit `PCIE` – enable Pin Change Interrupt which we use to process the IR remote control codes.

Pin change interrupt mask (`PCMSK`):

- bit `3` – Select only pin 3 for Pin Change Interrupt

To enable the PWM, the 1st bit is set in `DDRB`.

Timer/Counter is then initialized for PWM generation and IR pulse decoding. The Timer/Counter serves three purposes at the same time. First, it is used to drive the PWM on the `OC0B` (PB1) pin. Second, it is used to measure

the pulse widths for the pulse-period demodulation to decode the IR remote control signals. To measure the pulse lengths, we read the Timer/Counter value and store it in the variable `previous_TCNT0_value`. By calculating the difference between the current and the previous readings, we may evaluate the pulse period. As we carefully select the Timer/Counter frequency to 18.75 kHz (54 us per tick), pulse widths from 54 us to 14 ms can be measured. The NEC IR protocol uses pulse widths from 560 us to 9 ms. We also use the Timer overflow interrupt to hang up the IR code receive as soon as the timer overflows for the second time (14 to 28 ms after the last pulse has been transmitted). Third, Timer/Counter overflows are used to trigger periodic battery level checks.

Therefore, we choose the following settings for the Timer/Counter. The Fast PWM mode with 0xFF as TOP is selected, with generation of a Non-inverting signal on pin `OC0B`, which is the same pin as `PB1` aka PWM pin. In this mode, 8-bit clock counts from 0 to 255 and starts again at zero. When it encounters the value `OCR0B`, it clears the `OC0B` bit, and sets it high again when the counter is restarted from zero. The frequency is chosen to be 18.75 kHz (approx. 53.3 µs per tick), which is obtained by selecting 64 as Timer/Counter prescaler, i.e., divide system clock by 64 for the Timer/Counter frequency.

Timer/Counter control register A (`TCCR0A`):

- bits `WGM00` and `WGM01` – set Fast PWM mode with 0xFF as TOP;
- bit `COM0B1` – set Clear OC0B on Compare Match.

Timer/Counter control register B (`TCCR0B`):

- bit mask `0x3` – set 64 as Timer/Counter prescaler.

**C code**

```c
if(!battery_status_critical) {
    GIMSK = 1 << PCIE;
    PCMSK = 1 << BIT_IR;
    DDRB |= 1 << BIT_PWM;
    TCCR0A = (1 << WGM01)
           | (1 << WGM00)
           | (1 << COM0B1);
    TCCR0B = 3;
```

**Assembler code**

```asm
.LIDLE_MEAS_BATTERY_ABOVECRITICAL:
lds r24,battery_status_critical
cpse r24,__zero_reg__
rjmp .LSTARTUP_SEQUENCE2
rjmp .LMAINLOOP_ENTRY
.LSTARTUP_SEQUENCE2:
ldi r24, 0x20
out GIMSK, r24
ldi r24, 0x08
out PCMSK, r24
sbi DDRB, 1
ldi r24, 0x23
out TCCR0A, r24
ldi r24, 0x03
out TCCR0B, r24
```

*S3.7.0d – Motor self-test* Perform a quick self-test: briefly turn on the motor to full power and measure the loaded battery voltage. To achieve that, we explicitly set the Timer/Counter Duty cycle (`OCR0B`) to 255 (100% duty cycle) and execute `pwm_start`.

**C code**

```c
    OCR0B = 255;
    pwm_start();
    _delay_ms(50);
    adc_fire_once();
    ensure_battery_level_above_critical();
    pwm_stop();
```

**Assembler code**

```asm
ldi r24, 255
out OCR0B, r24
pwm_start
delay16bit_r24_r25 50
adc_fire_once
ensure_battery_level_above_critical r24
pwm_stop
```

*S3.7.0e – Third part of the startup sequence* At the third part of the startup sequence, periodic battery level checks are enabled by using the Timer/Counter overflow (i.e., the moment when the PWM opens the transistor - we want the loaded voltage for critical discharge checks) as the trigger event to start the voltage measurement. To achieve this, the following settings are loaded to the registers.

ADC control register B (`ADCSRB`):

- bit `ADTS2` – set Timer/Counter Overflow as the ADC Auto Trigger Source.

ADC control register A (`ADCSRA`):

- bit `ADATE` – set ADC Auto Trigger Enable.

Timer interrupt mask register (`TIMSK0`):

- bit `TOIE0` – set Timer/Counter Overflow Interrupt Enable.

**C code**

```
    ADCSRB = (1 << ADTS2);
    ADCSRA |= (1 << ADATE);
    TIMSK0 |= (1 << TOIE0);
    ADCSRA |= (1 << ADIE);
    _delay_ms(1000);
    led_on();
    sei();
}
```

**Assembler code**

```
ldi r24, 0x4
out ADCSRB, r24
sbi ADCSRA, ADATE
in r24, TIMSK0
ori r24, 0x2
out TIMSK0, r24
sbi ADCSRA, ADIE
delay24bit 1000 r25 r18 r24
led_on
sei
rjmp .LMAINLOOP_ENTRY
```

*S3.7.0f – Main loop* The main loop is normally running forever. It is only broken out of if the battery level falls below critical. The PWM and IR remote control command receives run asynchronously, as is the battery level periodic checking, which is performed at the Timer/Counter overflow events, i.e., once in approximately 14 ms.

**C code**

```
while (!battery_status_critical){
    _delay_ms(1000);
}
```

**Assembler code**

```
.LMAINLOOP:
delay24bit 1000 r25 r18 r24
.LMAINLOOP_ENTRY:
lds r24, battery_status_critical
tst r24
breq .LMAINLOOP
```

*S3.7.0g – Power-saving mode* In case the flag `battery_status_critical` becomes set, the main loop is terminated and the power-saving mode is automatically entered. In this case, the PWM output is forced to logical low, all interrupts are globally disabled by the `cli` instruction, Timer/Counter and ADC are stopped by writing zeros to the registers `TCCR0B` and `ADCSRA`. After that, an infinite loop is entered that only consists in blinking the LED for 50 ms each three seconds.

**C code**

```
pwm_stop();
cli();
TCCR0B = 0;
ADCSRA = 0;
led_off();
while (1){
    _delay_ms(3000);
    led_on();
    _delay_ms(50);
    led_off();
}
```

**Assembler code**

```
pwm_stop
cli
out TCCR0B, __zero_reg__
out ADCSRA, __zero_reg__
led_off
.LPOWERSAVE_LOOP:
delay24bit 3000 r25 r18 r24
led_on
delay16bit_r24_r25 50
led_off
rjmp .LPOWERSAVE_LOOP
```

### S3.8 – Timer/Counter overflow interrupt service routine

This interrupt service routine is executed at each Timer/Counter overflow. The following actions are performed. First, an ADC single conversion is implicitly triggered on hardware level, as specified by the ADC Auto-trigger setting. Next, the `timer_overflow_flag` is set if it has not previously been. In case the flag had previously been set and not cleared by a time interval measurement, it means that the Timer/Counter has overflown twice since the last measurement, making the next measurement meaningless. This situation is treated as an IR command timeout, and the received IR data is dropped.

**C code**

```
ISR(TIM0_OVF_vect){
  if(timer_overflow_flag){
    ir_hangup();
  } else {
    timer_overflow_flag = 1;
  }
}
```

**Assembler code**

```
__vector_3:
push_status
for_registers 24 24 push
lds r24, timer_overflow_flag
cpse r24, __zero_reg__
rjmp .LNOT_FIRST_OVERFLOW
ldi r24, 1
sts timer_overflow_flag, r24
rjmp .LVECTOR3_EPILOGUE
.LNOT_FIRST_OVERFLOW:
ir_hangup
.LVECTOR3_EPILOGUE:
for_registers 24 24 pop
pop_status
reti
.size  __vector_3, .-__vector_3
```

### S3.9 – ADC conversion complete interrupt service routine

This interrupt service routine is executed each time an ADC conversion is completed. The only action it performs is to compare the measured supply voltage with the critical level and set the `battery_status_critical` flag if the measured level is lower or equal.

**C code**

```
ISR(ADC_vect){
  ensure_battery_level_above_critical();
}
```

**Assembler code**

```
__vector_9:
push_status
for_registers 24 24 push
ensure_battery_level_above_critical r24
for_registers 24 24 pop
pop_status
reti
.size  __vector_9, .-__vector_9
```

### S3.10 – Pin change interrupt service routine

The logical pin change interrupt service routine is used to decode the IR remote control codes, as defined by the NEC protocol. First, the pulse-period modulated code is demodulated by measuring the pulse lengths using the Timer/Counter and analyzing them using a finite state automaton (FSA). After all 32 bits have been received, they are checked for validity and correct address, and, if these tests are passed, the PWM duty cycle corresponding to the command is set.

*S3.10.0a – State machine* As soon as the logical level on the IR receiver output changes, the state machine, which is implemented using a `switch` statement, is fired to analyze the current state, which is stored in the variable `ir_state`. In a correct code, a 9000 ms negative pulse must be followed by a 4500 ms positive pulse, which is in turn followed by 32 pulse pairs carrying the data bits, which can be either a (560 µs↓ + 1680 µs↑) for logical 1, or (560 µs↓ + 560 µs↑) for logical 0. An IR remote control also sends repeat codes if the key is held pressed, but this firmware effectively ignores them due to a timeout occurring in the absence of the data bits. If at any of the described states a wrong pulse length or polarity is found, the state machine is reset to the idle state, and the bit data is discarded.

Note: in assembler code, the edge type (one for rising and zero for falling) is stored in the register `r24`.

**C code**

```
ISR(PCINT0_vect){
  uint8_t is_rising_edge = ((PINB >> BIT_IR) & 1);
  switch(ir_state){
  case IR_STATE_IDLE:
        ...
  case IR_STATE_LEADING_9000ms:
        ...
  case IR_STATE_LEADING_4500ms:
        ...
  case IR_STATE_DATA_BITS:
        ...
  }
}
```

**Assembler code**

```
__vector_2:
push_status
for_registers 17 31 push
in r24, PINB
bst r24, BIT_IR
clr r24
bld r24, 0
lds r25, ir_state
cpi r25, IR_STATE_LEADING_9000ms
brne .+2
rjmp .LVECTOR2_CASE_IR_STATE_LEADING_9000ms
brsh .+2
rjmp .LVECTOR2_CASE_IR_STATE_IDLE
cpi r25, IR_STATE_LEADING_4500ms
breq .LVECTOR2_CASE_IR_STATE_LEADING_4500ms
cpi r25, IR_STATE_DATA_BITS
breq .LVECTOR2_CASE_IR_STATE_DATA_BITS
.LVECTOR2_EPILOGUE:
for_registers 31 17 pop
pop_status
reti
.size  __vector_2, .-__vector_2
```

*S3.10.0b – Changes from the idle state* As the IR receiver is pulled high, a transmission may only be started by a falling edge. If a transmission is started, reset the timer and the FSA is switched into the next state `IR_STATE_LEADING_9000ms`.

**C code**

```
case IR_STATE_IDLE:
    if(!is_rising_edge){
      start_time_interval_measurement();
      ir_state = IR_STATE_LEADING_9000ms;
    }
    return;
```

**Assembler code**

```
.LVECTOR2_CASE_IR_STATE_IDLE:
cpse r24,__zero_reg__
rjmp .LVECTOR2_EPILOGUE
start_time_interval_measurement r24
ldi r24, IR_STATE_LEADING_9000ms
sts ir_state, r24
rjmp .LVECTOR2_EPILOGUE
```

*S3.10.0c – Changes from the state `IR_STATE_LEADING_9000ms`* This state corresponds to waiting for the end of a 9000 ms leading negative pulse, therefore a change to any of the next states may only be triggered by a rising edge. If a rising edge is encountered, the time interval between the previous falling edge and the current rising edge is measured. If its length indeed falls into the 9000 µs ± 20% interval (approx. 170 Timer/Counter cycles), the FSA is switched to the next state `IR_STATE_LEADING_4500ms`. If a pulse of any other length has been observed, the state machine is reset to the `IR_STATE_IDLE` state.

**C code**

```
case IR_STATE_LEADING_9000ms:
    if(is_rising_edge){
        uint8_t time_interval =
    get_time_interval_since_last_measurement();
        if(time_interval > usec_to_cycles(9000,
                -F_CPU_ACCURACY_PERCENT)
        && time_interval < usec_to_cycles(9000,
                +F_CPU_ACCURACY_PERCENT)){
            ir_state = IR_STATE_LEADING_4500ms;
        } else {
            ir_state = IR_STATE_IDLE;
        }
    }
    return;
```

**Assembler code**

```
.LVECTOR2_CASE_IR_STATE_LEADING_9000ms:
tst r24
breq .LVECTOR2_EPILOGUE
get_time_interval_since_last_measurement r24 r25
set_cycles_from_usec 9000, F_CPU_ACCURACY_PERCENT
subi r24, (CYCLES_LO + 1)
cpi r24, (CYCLES_HI - CYCLES_LO - 1)
brsh .LVECTOR2_RESET_TO_IDLE
ldi r24, IR_STATE_LEADING_4500ms
sts ir_state,r24
rjmp .LVECTOR2_EPILOGUE

.LVECTOR2_RESET_TO_IDLE:
sts ir_state,__zero_reg__
rjmp .LVECTOR2_EPILOGUE
```

*S3.10.0d – Changes from the state `IR_STATE_LEADING_4500ms`* This state corresponds to waiting for the end of a 4500 ms leading positive pulse, therefore a change to any of the next states may only be triggered by a falling edge. If a falling edge is encountered, the time interval between the previous rising edge and the current falling edge is measured. If its length indeed falls into the 4500 µs ± 20% interval (approx. 85 Timer/Counter cycles), the `ir_shift_register` is emptied and the FSA is switched to the next state `IR_STATE_DATA_BITS`.

If a pulse of any other length has been observed, the state machine is reset to the `IR_STATE_IDLE` state.

### C code

```
  case IR_STATE_LEADING_4500ms:
    if(!is_rising_edge){
      uint8_t time_interval =
   get_time_interval_since_last_measurement();
      if(time_interval > usec_to_cycles(4500,
                     -F_CPU_ACCURACY_PERCENT)
      && time_interval < usec_to_cycles(4500,
                     +F_CPU_ACCURACY_PERCENT)){
        ir_state = IR_STATE_DATA_BITS;
        ir_received_bits_count = 0;
        ir_shift_register = 0;
        led_off();
      } else {
        ir_state = IR_STATE_IDLE;
      }
    }
    return;
```

### Assembler code

```
.LVECTOR2_CASE_IR_STATE_LEADING_4500ms:
cpse r24,__zero_reg__
rjmp .LVECTOR2_EPILOGUE
get_time_interval_since_last_measurement r24 r25
set_cycles_from_usec 4500, F_CPU_ACCURACY_PERCENT
subi r24, (CYCLES_LO + 1)
cpi r24, (CYCLES_HI - CYCLES_LO - 1)
brlo .+2
rjmp .LVECTOR2_RESET_TO_IDLE
ldi r24, IR_STATE_DATA_BITS
sts ir_state, r24
sts ir_received_bits_count,__zero_reg__
sts ir_shift_register,__zero_reg__
sts ir_shift_register+1,__zero_reg__
sts ir_shift_register+2,__zero_reg__
sts ir_shift_register+3,__zero_reg__
led_off
rjmp .LVECTOR2_EPILOGUE
```

*S3.10.0e – Changes from the state IR_STATE_DATA_BITS* This state corresponds to high logical level and waiting for a data pulse pair, which can be either a (560 µs↓ + 1680 µs↑) for logical 1, or (560 µs↓ + 560 µs↑), therefore a change to any of the next states may only be triggered by a falling edge. In this state, rising edges are skipped, and distances between falling edges are measured, thus yielding the total length of a pulse pair. If a falling edge is ignored, the time interval between the previous and the current falling edges is measured.

### C code

```
case IR_STATE_DATA_BITS:
    if(is_rising_edge){
       return;
    }
    uint8_t time_interval =
        get_time_interval_since_last_measurement();
    uint8_t new_bit;
    if(time_interval > usec_to_cycles(560 + 560,
            -F_CPU_ACCURACY_PERCENT)
    && time_interval < usec_to_cycles(560 + 560,
            +F_CPU_ACCURACY_PERCENT)){
        new_bit = 0;
    } else {
        if(time_interval > usec_to_cycles(560 + 1680,
                -F_CPU_ACCURACY_PERCENT)
        && time_interval < usec_to_cycles(560 + 1680,
                +F_CPU_ACCURACY_PERCENT)){
            new_bit = 1;
        } else {
            ir_hangup();
            return;
        }
    }
```

### Assembler code

```
.LVECTOR2_CASE_IR_STATE_DATA_BITS:
cpse r24,__zero_reg__
rjmp .LVECTOR2_EPILOGUE
get_time_interval_since_last_measurement r24 r25
set_cycles_from_usec (560+560), F_CPU_ACCURACY_PERCENT
ldi r25, (-CYCLES_LO - 1)
add r25, r24
cpi r25, (CYCLES_HI - CYCLES_LO - 1)
brsh .+2
rjmp .LVECTOR2_NEWBIT_ZERO
set_cycles_from_usec (1680+560), F_CPU_ACCURACY_PERCENT
subi r24, (CYCLES_LO + 1)
cpi r24, (CYCLES_HI - CYCLES_LO - 1)
brlo .+2
rjmp .LVECTOR2_IR_HANGUP
.LVECTOR2_NEWBIT_ONE:
ldi r20, 1
rjmp .LVECTOR2_STORE_NEW_BIT
.LVECTOR2_IR_HANGUP:
ir_hangup
rjmp .LVECTOR2_EPILOGUE
.LVECTOR2_NEWBIT_ZERO:
ldi r20, 0
.LVECTOR2_STORE_NEW_BIT:
```

If the obtained pulse length falls in the (560 µs ↓ +560 µs ↑) ± 20% interval, it is treated as a logical 0. If it falls in the (560 µs ↓ +1680 µs ↑) ± 20% interval, this pulse pair is treated as a logical 1. In either of the mentioned cases, the state machine remains in the `IR_STATE_DATA_BITS` waiting for the next data bit. If a pulse of any other length has been observed, the state machine is reset to the `IR_STATE_IDLE` state and all the received bits are dropped.

*S3.10.0f – Shifting the bits into `ir_shift_register`* The newly received data bit is shifted into `ir_shift_register`.

**C code**

```
ir_shift_register = (ir_shift_register << 1)
                  | new_bit;
ir_received_bits_count++;
```

**Assembler code**

```
.LVECTOR2_STORE_NEW_BIT:
lds r24,ir_shift_register
lds r25,ir_shift_register+1
lds r26,ir_shift_register+2
lds r27,ir_shift_register+3
lsl r24
rol r25
rol r26
rol r27
or r24, r20
sts ir_shift_register,r24
sts ir_shift_register+1,r25
sts ir_shift_register+2,r26
sts ir_shift_register+3,r27
lds r24,ir_received_bits_count
inc r24
sts ir_received_bits_count, r24
.LVECTOR2_CHECK_32BITS_RECEIVED:
```

*S3.10.0g – Checking if all 32 bits have been received*

**C code**

```
if(ir_received_bits_count == 32){
    ir_hangup();
    if ((ir_shift_register >> 16)
            != REMOTECONTROL_ADDRESS){
        return;
    }
    uint8_t command =
        (uint8_t) (ir_shift_register >> 8);
    uint8_t not_not_command =
        (uint8_t) ~((uint8_t) ir_shift_register);
    if (command != not_not_command) {
        return;
    }
```

**Assembler code**

```
.LVECTOR2_CHECK_32BITS_RECEIVED:
lds r24, ir_received_bits_count
cpi r24, 32
breq .+2
rjmp .LVECTOR2_EPILOGUE
ir_hangup
lds r24,ir_shift_register
lds r25,ir_shift_register+1
lds r26,ir_shift_register+2
lds r27,ir_shift_register+3
movw r20,r26
clr r22
clr r23
cpi r20, lo8(REMOTECONTROL_ADDRESS)
sbci r21, hi8(REMOTECONTROL_ADDRESS)
cpc r22, __zero_reg__
cpc r23, __zero_reg__
breq .+2
rjmp .LVECTOR2_EPILOGUE
mov r17,r25
com r24
cpse r25,r24
rjmp .LVECTOR2_EPILOGUE
.LVECTOR2_FIND_BUTTON:
```

After shifting a new data bit into `ir_shift_register`, a test is performed if all 32 data bits have been received. In case they have, the state machine is reset to the `IR_STATE_IDLE` state and the bit sequence is parsed.

It consists of 16 address bits (which may, in turn, consist of a 8 bit address followed by its logical inversion, but this is not always the case) followed by a 8-bit command, which is in turn followed by its logical inverse. We decode this here. We first verify that the address is correct (the command is from our remote control, i.e., directed to our bot, not to an air conditioner nor a projector), and then verify that `command == command_logical_inverse`, i.e., the command is a valid one.

*S3.10.0h – Finding known commands* In case all test have been passed, the command is searched in the list of known commands, and, if found, the corresponding duty cycle is set.

**C code**

```c
        uint8_t i;
        for (i = 0;
             i < sizeof(IR_REMOTE_CONTROL_BUTTONS)
                 / sizeof(ir_button_t);
             i++){
            ir_button_t maybe_this_button =
                IR_REMOTE_CONTROL_BUTTONS[i];
            if(command == maybe_this_button.command){
                pwm_set_duty_cycle(
                    maybe_this_button.pwm_duty_cycle
                );
            }
        }
    }
}
```

**Assembler code**

```asm
.LVECTOR2_FIND_BUTTON:
ldi r28,lo8(IR_REMOTE_CONTROL_BUTTONS)
ldi r29,hi8(IR_REMOTE_CONTROL_BUTTONS)
rjmp .LVECTOR2_LOOP_OVER_BUTTONS_ENTRY
.LVECTOR2_LOOP_OVER_BUTTONS:
adiw r28,2
ldi r24,hi8(IR_REMOTE_CONTROL_BUTTONS + 2*LIST_SIZE)
cpi r28,lo8(IR_REMOTE_CONTROL_BUTTONS + 2*LIST_SIZE)
cpc r29,r24
brne .+2
rjmp .LVECTOR2_EPILOGUE

.LVECTOR2_LOOP_OVER_BUTTONS_ENTRY:
ld r24,Y
cpse r17,r24
rjmp .LVECTOR2_LOOP_OVER_BUTTONS
ldd r24,Y+1
pwm_set_duty_cycle r24 .LVECTOR2_LOOP_OVER_BUTTONS
```

[1] ATTiny13/ATTiny13V: 8-bit AVR microcontroller with 1K bytes in-system programmable flash. Datasheet, Rev. 2535J-AVR-08/10, Atmel Corporation, https://ww1.microchip.com/downloads/en/devicedoc/doc2535.pdf. Accessed 22 May 2023.
